# Supplementary material for: MTV: Visual Analytics for Detecting, Investigating, and Annotating Anomalies in Multivariate Time Series
Source: arXiv:2112.05734 source file (2021-12-10)
Supplement: Supplementary file 1 [file appendix.tex]

\newpage

\section{Study Context: Time Series Anomaly Detection}
\label{sec:context}
An anomaly detection task requires an input sequence $\mathbf{x} = [\mathbf{x}^1, \mathbf{x}^2, \dots, \mathbf{x}^T]$, which we refer to as a time series of length $T$. 
Each data point $\mathbf{x}^i \in \mathbb{R}^m$ is a vector that represents a multi-channel measurement. 
To simplify our notation, we use $m=1$ (i.e., $x^i \in \mathbb{R}$) where $x^i$ is now a scalar. 
This notation follows the definition of a single-variate time series; however, the same process can be extrapolated to represent multivariate time series when $\mathbf{x}^i \in \mathbb{R}^m$. 

The objective is to produce an interval of timestamps ($t_s, t_e$), where $t_s, t_e \in [1, T]$ and $t_s \leq t_e$. 
A task can output several intervals that are suspected to be anomalous. 
Formally, we denote the output as an anomaly set $\mathbf{A}$ where $\mathbf{A} = \{(t_j, t_{j+w}) \:|\: 1 \leq j < T - w\}$ and $w$ resembles the anomalous window width. 
In our definition, $w$ differs in each anomalous interval.
For example, for $\mathbf{x}= [x^1, x^2, x^3, x^4, \dots, x^T]$ and assuming that the following data points $x^2, x^3, x^4$ are anomalous points, then $\mathbf{A} = \{(t^2, t^4)\}$ is the output of the anomaly detection process (note $w = 3$ in this example). 

In this work, we use unsupervised learning models to identify anomalies.
Unsupervised learning is a common approach for anomaly detection within time series, due to a lack of labeled data and shifting contexts that change what is considered an anomaly -- a dataset labeled in one context may not apply to the new context at hand.
For the rest of the paper, we will use "time series" and "signals" interchangeably to represent time-varying variables based on the context.
